# Supplementary material for: Uncertainty-aware Knowledge Tracing
Source: arXiv:2501.05415 source file (2025-01-21)
Supplement: Supplementary file 1 [file appendix.tex]

\begin{figure*}
		\centering % 表示居中
            \includegraphics[width=\linewidth]{UKT/picture/图片1.png}
		\caption{Performance on other four datasets with varying $\lambda$ values} \label{performance}
\end{figure*}
